# Supplementary material for: Fairness in Multi-Task Learning via Wasserstein Barycenters
Source: arXiv:2306.10155 source file (2023-07-06)
Supplement: Supplementary file 1 [file additional_results.tex]

% \begin{table*}[h!]%[h]
% \begin{normalsize}
%     \resizebox{\linewidth}{!}{
%     \begin{tabular}{|l||*{8}{c|}} \hline
%     \multirow{2}{*}{\begin{tabular}{p{0.5cm}}\backslashbox[30mm]{Data}{Model} 
%     \end{tabular}} & \multicolumn{2}{c|}{MTL} & \multicolumn{2}{c|}{MTL, Post-processed} & \multicolumn{2}{c|}{STL} &
%     \multicolumn{2}{c|}{STL, Post-processed}\\ \cline{2-9}
%      & Performance & Unfairness & Performance & Unfairness & Performance & Unfairness & Performance & Unfairness \\ \hline\hline
%     regression - all data & 
%     $0.548 \pm 0.02$ & 
%     $0.109 \pm 0.01$ &
%     $0.558 \pm 0.02$ &
%     $0.018 \pm 0.00$ &
%     $0.559 \pm 0.02$ &
%     $0.107 \pm 0.01$ &
%     $0.572 \pm 0.02$ & 
%     $0.018 \pm 0.01$ \\
%     regression - 25\% missing &
%     $0.558 \pm 0.02$ & 
%     $0.109 \pm 0.02$ & 
%     $0.572 \pm 0.02$ & 
%     $0.018 \pm 0.00$ & 
%     $0.570 \pm 0.02$ & 
%     $0.105 \pm 0.02$ & 
%     $0.583 \pm 0.02$ & 
%     $0.018 \pm 0.01$ \\
%     regression - 50\% missing &
%     $0.577 \pm 0.02$ & 
%     $0.109 \pm 0.02$ & 
%     $0.593 \pm 0.03$ & 
%     $0.018 \pm 0.01$ & 
%     $0.587 \pm 0.02$ & 
%     $0.099 \pm 0.01$ & 
%     $0.601 \pm 0.02$ & 
%     $0.018 \pm 0.01$ \\
%    % \hline
%     regression - 75\% missing &
%     $0.612 \pm 0.05$ & 
%     $0.101 \pm 0.02$ & 
%     $0.627 \pm 0.06$ & 
%     $0.019 \pm 0.01$ & 
%     $0.632 \pm 0.04$ & 
%     $0.098 \pm 0.01$ & 
%     $0.645 \pm 0.04$ & 
%     $0.019 \pm 0.00$ \\
%     regression - 95\% missing &
%     \cellcolor{blue!15}$0.678 \pm 0.05$ & 
%     $0.105 \pm 0.02$ & 
%     \cellcolor{blue!15}$0.687 \pm 0.05$ & 
%     $0.018  \pm 0.01$ & 
%     $0.738 \pm 0.06$ & 
%     $0.108 \pm 0.03$ & 
%     $0.750 \pm 0.05$ & 
%     $0.018 \pm 0.01$ \\
%     \hline
%     classification - all data & 
%     $0.576 \pm 0.01$ & 
%     $0.080  \pm 0.03$ & 
%     $0.577 \pm 0.01$ & 
%     $0.018 \pm 0.01$ & 
%     \cellcolor{blue!15}$0.640 \pm 0.03$ & 
%     $0.042 \pm 0.02$ & 
%     \cellcolor{blue!15}$0.640 \pm 0.03$ & 
%     $0.018 \pm 0.01$ \\
%     \hline
%     \hline
%     \end{tabular}}
%     \vspace{0.1cm}
%     \caption{Performance (MSE for regression task, AUC for classification) and unfairness for MTL and Single Task Learning (STL) Models. Each model was also post-processed and evaluated on performance and unfairness.}
%     \label{table:resultsfolk}
%     \end{normalsize}
% \end{table*}
